# Supplementary material for: A geometrically aware auto-encoder for multi-texture synthesis
Source: arXiv:2302.01616 source file (2023-06-29)
Supplement: Supplementary file 1 [file 12_appendix.tex]

\label{sec:appendix}

\newcommand{\figa}{9}
\newcommand{\figb}{16}
\newcommand{\figc}{15}
\newcommand{\figd}{29}
\newcommand{\fige}{35}
\newcommand{\figg}{12}

\begin{figure*}
\centering
\begin{tabular}{cccccc}
\setlength{\tabcolsep}{.1pt}

\centering
GT & TAE (ours) & WCT & TextureCNN & Neural Texture  \\

\includegraphics[width=.2\linewidth]{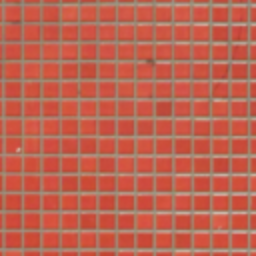}&
\includegraphics[width=.2\linewidth]{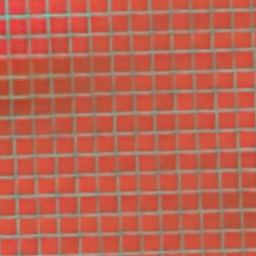}&
\includegraphics[width=.2\linewidth]{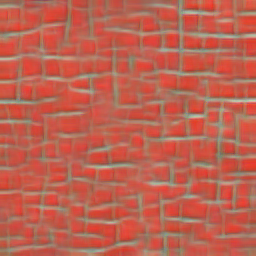}&
\includegraphics[width=.2\linewidth]{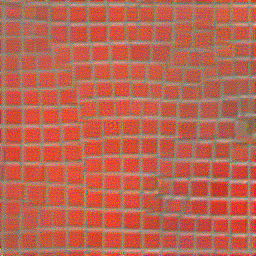}&
\includegraphics[width=.2\linewidth]{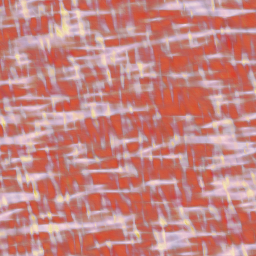} \\

\includegraphics[width=.2\linewidth]{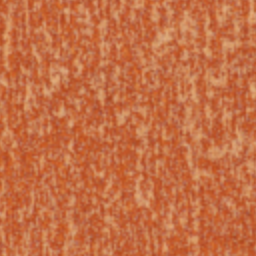}&
\includegraphics[width=.2\linewidth]{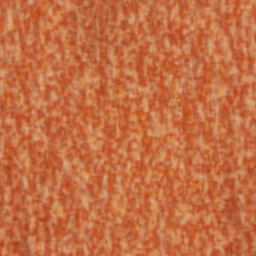}&
\includegraphics[width=.2\linewidth]{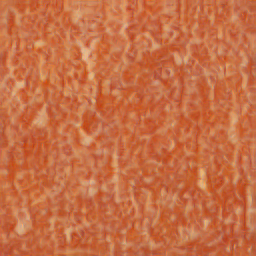}&
\includegraphics[width=.2\linewidth]{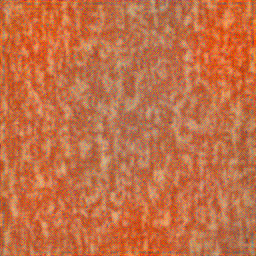}&
\includegraphics[width=.2\linewidth]{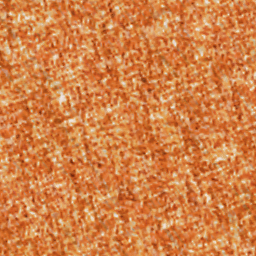} \\

\includegraphics[width=.2\linewidth]{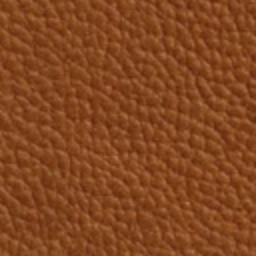}&
\includegraphics[width=.2\linewidth]{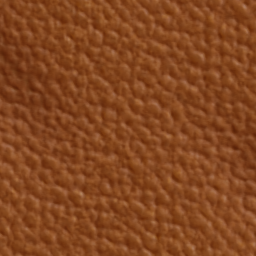}&
\includegraphics[width=.2\linewidth]{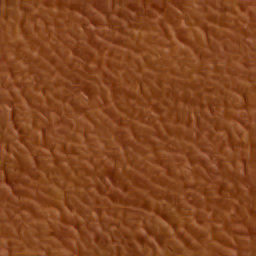}&
\includegraphics[width=.2\linewidth]{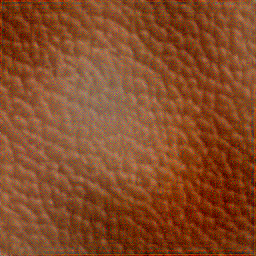}&
\includegraphics[width=.2\linewidth]{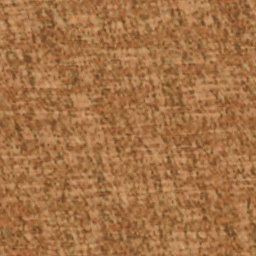} \\

\includegraphics[width=.2\linewidth]{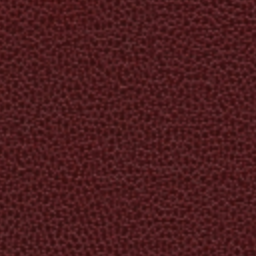}&
\includegraphics[width=.2\linewidth]{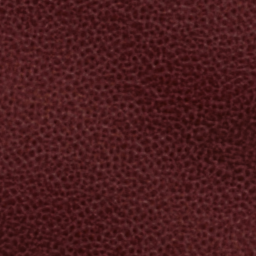}&
\includegraphics[width=.2\linewidth]{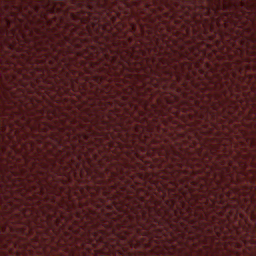}&
\includegraphics[width=.2\linewidth]{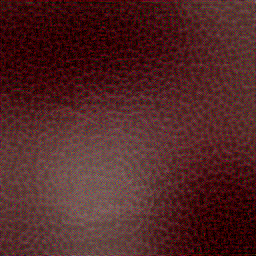}&
\includegraphics[width=.2\linewidth]{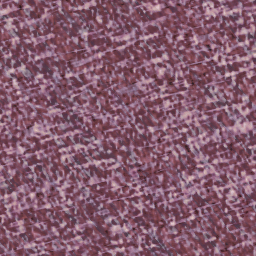} \\

\includegraphics[width=.2\linewidth]{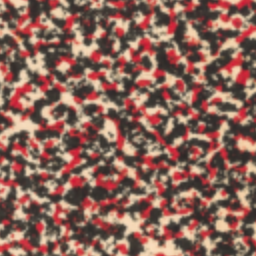}&
\includegraphics[width=.2\linewidth]{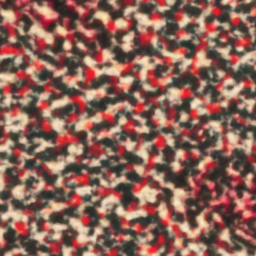}&
\includegraphics[width=.2\linewidth]{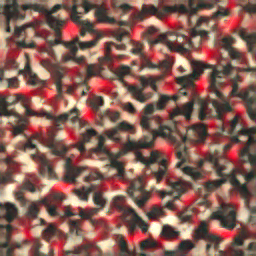}&
\includegraphics[width=.2\linewidth]{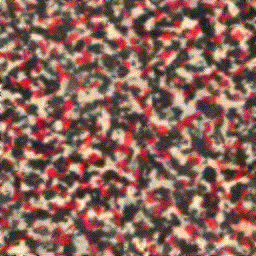}&
\includegraphics[width=.2\linewidth]{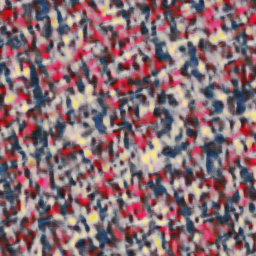} \\

\includegraphics[width=.2\linewidth]{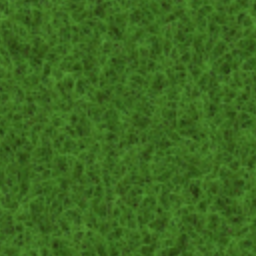}&
\includegraphics[width=.2\linewidth]{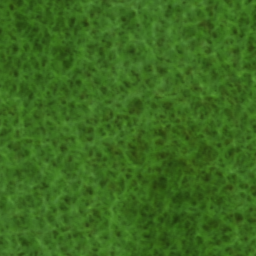}&
\includegraphics[width=.2\linewidth]{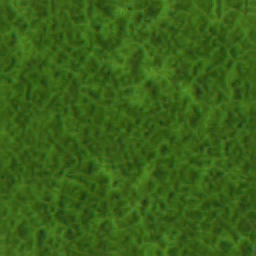}&
\includegraphics[width=.2\linewidth]{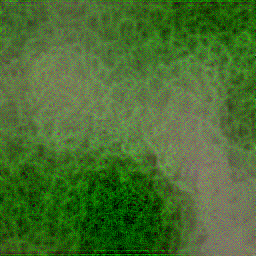}&
\includegraphics[width=.2\linewidth]{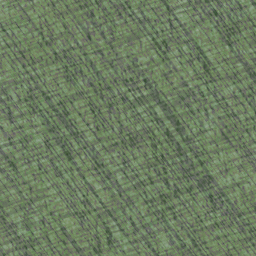} \\

\end{tabular}
\caption{Comparison of syntheses obtained from the 5 different methods.}
\label{comp_fig}
\end{figure*}
% \section{}
